# Supplementary material for: K-motives, Springer Theory and the Local Langlands Correspondence
Source: arXiv:2401.13052 source file (2024-01-28)
Supplement: Supplementary file 1 [file appendix.tex]

\appendix
\section{Introduction}
We explain how the \emph{Riemann--Roch map} naturally arises from a general framework of bivariant motivic cohomology theories and orientations, as developed in \cite{degliseBivariantTheoriesMotivic2018,degliseOrientationTheoryArithmetic2019}. We follow the notation in \emph{loc. cit.}

{\color{red} WRITE THIS}
\section{Background on generalized motivic cohomology}
\subsection{Cohomology theories from absolute ring spectra}Let $\E\in\Tt$ be an absolute ring spectrum in a motivic triangulated category. \emph{Cohomology} and \emph{Borel--Moore homology} associated to $\E$ is defined by
\begin{align*}
    \E^{n,m}(X)&=\Hom_{\Tt(X)}(\un_X,\E_X(m)[n])\text{ and}\\
    \E^{BM}_{n,m}(X/S)&=\Hom_{\Tt(X)}(\un_X(m)[n],f^!\E_S).
\end{align*}
where $X$ is a scheme and $f:X\to S,$ a morphism.
Borel--Moore homology is a bivariant theory in the sense of \cite{fultonCategoricalFrameworkStudy1981} and is contravariant with respect to maps $T\to S$ and covariant with respect to proper maps $Y\to X.$

For a morphism $f:X\to S$ A \emph{fundamental class} of dimension $d$ is a morphism
$$\eta: \E_X(d)[2d]\to f^!\E_S.$$
Given a class of morphisms closed under composition, a \emph{system of fundamental classes} is a choice of fundamental classes $\eta_f$ for each morphism in this class, such that $\eta_{fg}^\E=\eta_{g}^\E\eta_{f}^\E.$

\subsection{Oriented Ring Spectra}
Let $\E\in\Tt$ be an absolute ring spectrum. Then, for every scheme $S$ there is a natural isomorphism
$$\tilde \E^{2,1}(\Proj^1_S)\stackrel{\sim}{\to} \E^{0,0}(S).$$
The \emph{stability class} $\sigma_S^\E\in \E^{2,1}(\Proj^1_S)$ is the preimage of the unit of the ring spectrum $(\un_S\stackrel{\eta_S}{\to} \E_S)\in \E_S^{0,0}$ under this isomorphism.

An \emph{orientation} $c$ of a ring spectrum is a choice of a class $c_S\in \E^{2,1}(\Proj^\infty_S)$ for each smooth $S$ such that $c_S$ restricts to $\sigma_S$ on $\Proj^1_S$ and $f^*(c_S)=c_T$ for $f:T\to S.$

Orientations are closely related to characteristic classes. For example, they allow to define the first Chern class
\begin{equation}\label{eq:chernclassfromorientation}
c_1: \Pic(S)\to \E^{2,1}(S)
\end{equation}
and, if $\E$ satisfies the projective bundle formula, higher Chern classes.

To an oriented absolute ring spectrum $(\E,c)$ one can associate a system of fundamental classes $\eta^{c}_f$ for the class of \emph{gci morphisms}\footnote{This includes morphisms which factor into a smooth map and regular immersion.} 
$f:X\to S$ by \cite[Theorem 2.5.3]{degliseBivariantTheoriesMotivic2018}.
The construction of the fundamental classes in \emph{loc.\ cit.\@}\ relies on the deformation to the normal cone diagram
\begin{equation}\label{eq:deformationtothenormalcone}
\begin{tikzcd}
    Z \arrow[r] \arrow[d] & \A^1_Z \arrow[d] & Z \arrow[l] \arrow[d] \\
    X \arrow[r, "d_1"] & D_Z X & N_Z X \arrow[l, "d_0"']
\end{tikzcd}
\end{equation}
which deforms a regular pair $(X,Z)$ (so $Z\to X$ is a regular immersion) to the normal bundle with zero section $(N_ZX,Z).$
\subsection{Duality and Gysin morphism}
An absolute ring spectrum $\E$ is called \emph{absolutely pure} if for each regular pair $(X,Z)$ where $X$ is also regular, the cohomology theory $\E$ admits the Thom isomorphism via the deformation diagram \eqref{eq:deformationtothenormalcone}, that is, the following maps are isomorphisms
$$\E^{*,*}_Z(X)=\E^{*,*}(X, Z) \overset{d_1^*}{\leftarrow} \E^{*,*}(D_{Z}X, \A^1_{Z}) \overset{d_2^*}{\rightarrow} \E^{*,*}(N_{Z}X, Z) = \E^{*,*}(\Th(N_{Z}X)).$$
For an oriented absolute ring spectrum $(\E,c)$ which is absolutely pure, the fundamental classes $\eta^{c}_f$ are actually isomorphisms and be can be used to express various versions of Poincar\'e duality. For example, the \emph{duality map}
\begin{equation}\label{eq:dualityforborelmoore}\delta^{c}_f\colon\E^{BM}_{n,m}(X/Y)\to \E^{BM}_{2d+n,d+m}(X/S), x\mapsto x\eta_f^{c}\end{equation}
is an isomorphism, for $f:Y\to S$ a gci-morphism of relative dimension $d$  and any scheme $X/Y.$ Moroever, for any gci-morphism $f:X\to Y$ of relative dimension $d$ we obtain the (functorial) \emph{Gysin morphism}
\begin{equation}\label{eq:gysinggci}f^!\colon\E^{BM}_{n,m}(Y/S)\to \E^{BM}_{2d+n,d+m}(X/S), y\mapsto y\eta_f^{c}.\end{equation}
For a Cartesian square with $i$ a regular closed immersion,
\[\begin{tikzcd}[sep=0pt]
	{X'} && {Y'} \\
	& \Delta \\
	X && Y
	\arrow["g"', from=1-1, to=3-1]
	\arrow["i'", from=1-1, to=1-3]
	\arrow["f", from=1-3, to=3-3]
	\arrow["i", from=3-1, to=3-3]
\end{tikzcd}\]
the \emph{refined fundamental class} and \emph{refined Gysin morphism} are defined by 
\begin{align}
	\label{eq:refinedfundamental}
	\eta^{c}_\Delta&=\Delta^*(\eta_p^c)\in \E^{BM}(X'/Y')\text{ and }\\
	\label{eq:refinedgysin}
	\Delta^!&\colon \E^{BM}_{n,m}(Y'/S)\to \E^{BM}_{2d+n,d+m}(X'/S),\, y\mapsto y\eta_\Delta^c.
\end{align}
The refined fundamental class and Gysin map depend on the Cartesian diagram $\Delta$ as opposed to just the map $X'\to Y'$ and fulfills, amongst others, the following properties.
\begin{lemma}
For a diagram Cartesian squares where $i$ and $j$ are gci
\[\begin{tikzcd}[sep=0pt]
	{X''} && {Y''} \\
	& {\Delta''} \\
	{X'} && {Y'} && {Z'} \\
	& \Delta && {\Delta'} \\
	X && Y && Z
	\arrow["f"', from=3-1, to=5-1]
	\arrow["g", from=3-3, to=5-3]
	\arrow["i", from=5-1, to=5-3]
	\arrow["{f'}"', from=1-1, to=3-1]
	\arrow["{g'}", from=1-3, to=3-3]
	\arrow["{i''}", from=1-1, to=1-3]
	\arrow["{i'}", from=3-1, to=3-3]
	\arrow["{j'}", from=3-3, to=3-5]
	\arrow["j", from=5-3, to=5-5]
	\arrow["h", from=3-5, to=5-5]
\end{tikzcd}\]
we denote by $\Delta'\Delta$ and $\Delta\Delta''$ the Cartesian squares obtained by horizontal and vertical composition, respectively. Then the following statements hold.
\begin{enumerate}
	\item Projection formula: For $g'$ proper, $f'_*(\Delta''\Delta)^!=\Delta^!g'_*.$
	\item Functoriality: $\Delta^!\Delta'^!=(\Delta'\Delta)^!$ and $\Delta^!=\id$ if $i=\id$.
	\item If $i,i'$ are gci of the relative dimension, $(\Delta\Delta'')^!=\Delta''^!.$
\end{enumerate}
\end{lemma}

\section{Correspondences and pure motives}
For an absolutely oriented absolute ring spectrum $(\E,c)$ we define categories of (relative) correspondences and pure $(\E,c)$-motives. This is a generalization of the category $\op{CHM}$ of pure Chow motives defined in \cite{cortiMotivicDecompositionIntersection2000} where $\E^{BM}_{2n,n}=\CH_n$ are Chow groups.
\subsection{The category of correspondences} 
Let $S/B$ be a scheme over regular base scheme. We abbreviate $X\times Y=X\times_B Y$ and $XY=X\times_SY.$
The category of $(\E,c)$-correspondences over $S/B$ denoted by $\Corr_{(\E,c)}(S/B)$ has objects proper morphisms $p:X\to S$ (which we often just denote by $X$) such that $X$ is smooth over $B$ and morphisms given by $\E$-correspondences\todo{This way the composition of morphisms is the wrong way around. Turn everything around.}
$$\Hom_{\Corr_{(\E,c)}(S/B)}(X,Y)=\bigoplus_{\alpha}\E^{BM}_{2d_X,d_X}(XY/B)$$
where $X/B$ has dimension\footnote{For simplicity, we only treat the equidimensional case here.} $d_X.$
Composition of morphisms is defined via the convolution product $$\E^{BM}_{2d_X,d_X}(XY/B)\times \E^{BM}_{2d_Y,d_Y}(YZ/B)\to \E^{BM}_{2d_X,d_X}(XZ/B),\,\alpha\circ\beta=p_{Y,*}\Delta_Y^!(\alpha\boxtimes\beta)$$ where $\Delta_Y$ is the refined Gysin morphism, see \eqref{eq:refinedgysin}, and $p_Y$ the proper pushforward associated to the diagram
\begin{equation}
	\label{eq:compositiondiagram}
	\begin{tikzcd}[column sep=0pt, row sep = 0pt]
	{XY\times YZ} && XYZ && XZ \\
	& \Delta_Y \\
	{X\times Y\times Y\times Z} && {X\times Y \times Z.}
	\arrow[from=1-3, to=1-1]
	\arrow["p_Y", from=1-3, to=1-5]
	\arrow[from=1-3, to=3-3]
	\arrow[from=3-3, to=3-1]
	\arrow[from=1-1, to=3-1]
\end{tikzcd}
\end{equation}
The refined Gysin map $\Delta_Y^!$ is well-defined, since the lower horizontal map in \eqref{eq:compositiondiagram} is a regular immersion: $Y\to Y\times Y$ is a regular immersion since $Y$ is smooth over $B$ and regularity is preserved by flat base change.
The following Lemma shows that this really defines a category.
\begin{lemma} Consider three morphisms $$\alpha\in \E^{BM}_{2d_W,d_W}(WX/B),\, \beta\in \E^{BM}_{2d_X,d_X}(XY/B)\text{ and }\gamma\in \E^{BM}_{2d_Y,d_Y}(YZ/B)$$
	in  $\Corr_{(\E,c)}(S/B).$ Let $\delta_X:X\to X\times_SX$ and $f_X:X\to B$ be the inclusion and the structure map. Denote $1_X=\delta_{X,*}(\eta_{f_X}^c)\in \E^{BM}_{2d_X,d_X}(XX/B).$
Then the following statements hold:
	\begin{enumerate}
		\item $\alpha\circ 1_X=\alpha$ and $1_X\circ\gamma=\gamma$ and
		\item $(\alpha\circ\beta)\circ \gamma=\alpha\circ(\beta\circ\gamma).$
	\end{enumerate}
\end{lemma}
\begin{proof}
\cite{fultonIntersectionTheory1998} \todo{ref correct lemma}
We leave (1) to the reader. For (2), consider the chain of equalities
\begin{align*}
	(\alpha\circ\beta)\circ\gamma&=p_{Y,*}\Delta_Y^!(p_{X,*}\Delta_X^!(\alpha\boxtimes\beta)\boxtimes\gamma)\\
	&=p_{Y,*}\Delta_Y^!(p_X\times\id_{YZ})_*(\Delta_X^!(\alpha\boxtimes\beta)\boxtimes\gamma)\\
	&=p_{Y,*}q_{X,*}\Delta_Y^{(b),!}(\Delta_X^!(\alpha\boxtimes\beta)\boxtimes\gamma)\\
	&=p_{Y,*}q_{X,*}\Delta_Y^{(c),!}\Delta_X^{(a),!}(\alpha\boxtimes\beta\boxtimes\gamma)\\
	
	&=q_*\Delta^!(\alpha\boxtimes\beta\boxtimes\gamma).
\end{align*}
The third equality follows from the projection formula for
\[\begin{tikzcd}[sep=0pt]
	{WXY\times YZ} && WXYZ \\
	& {\Delta^{(a)} _Y} \\
	{WY\times YZ} && WYZ && WZ \\
	& {\Delta_Y} \\
	{W\times Y\times Y\times Z} && {W\times Y \times Z}
	\arrow[from=3-1, to=5-1]
	\arrow[from=3-3, to=3-1]
	\arrow[from=3-3, to=5-3]
	\arrow[from=5-3, to=5-1]
	\arrow["{p_X\times\id_{YZ}}"', from=1-1, to=3-1]
	\arrow["{q_X}"', from=1-3, to=3-3]
	\arrow[from=1-3, to=1-1]
	\arrow["{p_Y}"', from=3-3, to=3-5]
	\arrow["q", from=1-3, to=3-5]
\end{tikzcd}\]
where we denote the vertical composition of the two squares by $\Delta^{(b)}_Y=\Delta_Y\Delta_Y^{(a)}.$ The fourth equality follows by staring at the diagram
\[\begin{tikzcd}[column sep=-3pt, row sep=0pt]
	{WX\times XY\times YZ} && {WXY\times YZ} && WXYZ \\
	& {\Delta^{(a)}_X} && {\Delta^{(c)}_Y} \\
	{W\times X\times X\times Y\times Y\times Z} && {W\times X\times Y\times Y\times Z} && {W\times X\times Y \times Z} \\
	&&& {\Delta^{(d)}_Y} \\
	&& {W\times Y\times Y\times Z} && {W\times Y \times Z.}
	\arrow[from=5-5, to=5-3]
	\arrow[from=1-5, to=1-3]
	\arrow[from=3-3, to=5-3]
	\arrow[from=3-5, to=5-5]
	\arrow[from=3-5, to=3-3]
	\arrow[from=1-3, to=1-1]
	\arrow[from=3-3, to=3-1]
	\arrow[from=1-1, to=3-1]
	\arrow[from=1-5, to=3-5]
	\arrow[from=1-3, to=3-3]
\end{tikzcd}\]
First, use that $\Delta_Y^{(b),!}=(\Delta_Y^{(c)}\Delta_Y^{(d)})^!=\Delta_Y^{(c),!}$ since the horizontal maps in $\Delta_Y^{(d)}$ are regular embeddings of the same relative dimension. Secondly, use that $\Delta^{(a),!}_X=\Delta_X^!\otimes\id.$\todo{fundamental class and exterior product}
For the last equality, we write $\Delta=\Delta_X^{(a)}\Delta_Y^{(c)}$ for the horizontal composition.

By symmetry, the same equality holds for $\alpha\circ(\beta\circ\gamma).$
\end{proof}
\begin{remark} The associativity also follows from \Cref{thm:embeddingpureintoall}.
\end{remark}
\subsection{Pure motives}
The category $\Corr_{(\E,c)}(S/B)$ is additive via disjoint union $X\oplus Y=X\sqcup Y$. We obtain the category of \emph{effective pure $\E$-motives}  $$\Pure_{(\E,c)}(S/B)_{eff}=\Kar(\Corr_{(\E,c)}(S/B))$$ by passing to the idempotent completion. So objects in $\Pure_{(\E,c)}(S/B)_{eff}$ are tuples $(p:X\to S, P)$ where 
$$P=P^2\in \Hom_{\Corr_{(\E,c)}(S/B)}(X,X)=\E^{BM}_{2d_X,d_X}(XX/B)$$
and morphisms are defined via the obvious commutative diagrams.

Lastly, the category of \emph{pure $\E$-motives} $$\Pure_{(\E,c)}(S/B)=\Pure_{(\E,c)}(S/B)_{eff}[\bL\inv]$$ is obtained by formally `inverting the Lefschetz motive $\bL$', which amounts to passing to triples $(p:X\to S, P, a)$ where $a$ is an integer and defining morphisms via
\begin{align*}
    \Hom_{\Pure_{(\E,c)}(S/B)}((X,P,a),(Y,Q,b))=P\E^{BM}_{2(d_X-a+b),d_X-a+b}(XY/B)Q.
\end{align*}

\section{$\E$-motives}
\subsection{Categories of $\E$-motives} For an absolute ring spectrum in a motivic triangulated category $\E\in \Tt$ the category of \emph{$\E$-motives} $$\DE{\E}=\Mod_\E(\Tt)$$ assigns to a scheme $X$ the category $\DE{\E}(X)=\Mod_{\E_X}(\Tt(X)).$ 

The category $\DE{\E}$ is again a motivic triangulated category and hence equipped with a six functor formalism using \todo{Cite CD}.
Cohomology and Borel--Moore homology with respect to $\E$ arise as
\begin{align*}
    \E^{n,m}(X)&=\Hom_{\DE\E(X)}(\un_X,\un_X(m)[m])\text{ and}\\
    \E^{BM}_{n,m}(X/S)&=\Hom_{\DE\E(X)}(\un_X(m)[n],f^!\un_S).
\end{align*}

The (stable $\infty$-)category of $\E$-motives is related to the additive (ordinary) category of pure $\E$-motives via the following theorem.
\begin{theorem}\label{thm:embeddingpureintoall} If $(\E,c)$ is an absolutely pure and oriented, then there is a fully faithful functor
$$\Ff_{(\E,c)}:\Corr_{(\E,c)}(S/B)\stackrel{\sim}{\hookrightarrow} \ho\DE\E(S)$$
which is defined on objects via $(p:X\to S)\mapsto p_!\un_X.$
\end{theorem}
\begin{proof} On morphisms the functor $\Ff_{(\E,c)}$ is defined by transversing the following diagram from the top right to the bottom left
\[\begin{tikzcd}
	& {\Hom_{\Corr_{(\E,c)}(S/B)}(X, Y)} \\
	{\E^{BM}_{0,0}(XY/Y)} & {\E^{BM}_{2d_2,d_2}(XY/B)} \\
	{\Hom_{\DE\E(XY)}(\pi_X^*\un_{X},\pi_Y^!\un_{Y})} & {\Hom_{\DE\E(XY)}(\pi_X^*\un_{X},f_{XY}^!\un_{B})} \\
	{\Hom_{\DE\E(Y)}(p_{X,*}\un_{X},p_{Y,!}\un_{Y})}
	\arrow["{(BC)}", Rightarrow, no head, from=4-1, to=3-1]
	\arrow[Rightarrow, no head, from=3-1, to=2-1]
	\arrow["{\delta^c_{f_Y}}", from=2-1, to=2-2]
	\arrow[Rightarrow, no head, from=1-2, to=2-2]
	\arrow["\sim", from=3-1, to=3-2]
	\arrow[Rightarrow, no head, from=2-2, to=3-2]
\end{tikzcd}\]
where $f_{XY}:XY\to B$ and $f_Y:Y\to B$ denote the projections, $\delta^{c}_{f_Y}$ is the duality map, see \eqref{eq:dualityforborelmoore} and $(BC)$ indicates base change for the Cartesian diagram
\[\begin{tikzcd}
	XY & Y \\
	X & S
	\arrow["{p_X}"', from=2-1, to=2-2]
	\arrow["{p_Y}", from=1-2, to=2-2]
	\arrow["{\pi_Y}", from=1-1, to=1-2]
	\arrow["{\pi_X}"', from=1-1, to=2-1]
\end{tikzcd}\]
To show that $\Ff_{(\E,c)}$ is compatible with composition we refer to \cite[Proposition 2.39]{fangzhouBorelMooreMotivic2016} where this is shown in the example $\DE{\E}=\DM.$ The same proof applies here.
\end{proof}
Since $\DE{\E}$ is idempotent complete\todo{reference} we can extend $\Ff_{(\E,c)}$ to pure $\E$-motives.
\begin{corollary} There is a fully faithful functor $$\Ff_{(\E,c)}:\Pure_{(\E,c)}(S/B)\hookrightarrow\ho\DE\E(S)$$ defined on objects via $$(p:X\to S,P,a)\mapsto \im(\Ff_{(\E,c)}(P):p_!\un_X\to p_!\un_X) (a)[2a].$$
\end{corollary}
\subsection{Weight Structures} Under certain $\op{Ext}$-vanishing assumptions, we may regard pure $(\E,c)$-motives as the pure objects with respect to \emph{weight structure} on a subcategory of $\DE{\E}$.
\begin{definition} The category of \emph{$(S/B)$-constructible $\E$-motives on $S$}
$$\DE{\E}_{(S/B)\! \op{-c}}(S)\subset \DE{\E}(S)$$
is the stable thick subcategory of $\DE{\E}(S)$ generated by objects of the form $p_!\un_X$ for $X\to S$ proper such that $X$ is smooth over $B$.
\end{definition}
\begin{theorem}\label{thm:existenceofweightstructure} Assume that
	$\E^{BM}_{2a-n,a}(XY/B)=0$ for all $X\to S, Y\to S$ proper, such that  $X$ and $Y$ are smooth over $S$ and $n\geq 0.$ Then there is a unique weight structure on $\DE{\E}_{(S/B)\! \op{-c}}(S)$ whose heart $\DE{\E}_{(S/B)\! \op{-c}}(S)^{w=0}$ is the thick subcategory generated by $p_!\un_X(a)[2a]$ for $X\to S$ proper such that $X$ is smooth over $B$ and $a\in \Z.$ Moreover, the functor $\Ff_{(\E,c)}$ restricts to an equivalence of categories
	$$\Ff_{(\E,c)}: \ho\DE{\E}_{(S/B)\! \op{-c}}(S)^{w=0}\to \Pure_{(\E,c)}(S/B).$$
\end{theorem}
\begin{proof} \todo{Reference Bondarko, generating weight structures}
\end{proof}

In particular, we obtain the \emph{weight complex functor}\todo{reference sosnilo for the definition}
$$\DE{\E}_{(S/B)\! \op{-c}}(S)\to \Ch^b(\ho\DE{\E}_{(S/B)\! \op{-c}}(S)^{w=0})\stackrel{\sim}{\to}\Ch^b(\Pure_{(\E,c)}(S/B))$$
which allows to express a general $\E$-motive in terms of pure motives.
\section{Change of Ring Spectra and the Riemann--Roch functor}
We now explain how (pure) motives if the underlying cohomology theory is changed.
\subsection{Change of orientations and Todd classes}
Let $\phi:\E\to \F$ be a morphism of absolute ring spectra in a motivic triangulated category $\Tt.$ This induces a functor between the motivic triangulated categories $\phi_*:\DE\E\to\DE\F$ as well as morphisms
\begin{align*}
    \phi_*:\E^{n,m}(X)&\to\F^{n,m}(X)\text{ and }
    \phi_*:\E^{BM}_{n,m}(X/S)\to\F^{BM}_{n,m}(X/S).
\end{align*}
Given orientations of the spectra $(\E,c)$, $(\F,d)$ we obtain the commutative diagram
\[\begin{tikzcd}
	{\E^{*,*}(\Proj^\infty_S)} & {\F^{*,*}(\Proj^\infty_S)} \\
	{\E^{*,*}(S)[[u]]} & {\F^{*,*}(S)[[t]]}
	\arrow["{\phi_*}", from=1-1, to=1-2]
	\arrow["\wr"', from=2-1, to=1-1]
	\arrow["\wr", from=2-2, to=1-2]
	\arrow[from=2-1, to=2-2]
\end{tikzcd}\]
where the vertical maps are induced by the orientations $u\mapsto c$ and $t\mapsto d$ and are isomorphisms via the projective bundle formula. The power series $\Psi_\phi(t)\in \F^{*,*}(S)[[t]]$ is defined as the image of $u$ under this map.
Since the map $\phi_*$ restricted to $\Proj^0_S$ is the zero map and restricted to $\Proj^1_S$ the identity (since it preserves the stability class), we obtain
$$\Psi_\phi(t)=t+\sum_{i>1}\alpha_it^i$$
and $\Psi_\phi(t)/t$ is invertible. By the splitting principle, there is a unique morphism of presheaves of abelian groups, associating to every vector bundle its \emph{Todd class}
$$\Td_\phi: K_0\to \F^{0,0,\times}$$
which satisfies for every line bundle $L/S$
$$\Td_\phi(L)=\frac{t}{\Psi_\phi(t)}d_1(L)$$
where $d_1$ denotes the Chern class associated to the orientation $d,$ see \eqref{eq:chernclassfromorientation}.

If $\E$, $\F$ are absolutely pure, by \cite[Theorem 3.2.6]{degliseBivariantTheoriesMotivic2018}, for any gci morphism $f:X\to S$ with virtual tangent bundle $\tau_f$, one has 
\begin{align}\label{eq:toddclassandfundamentalclasses}
    \phi_*(\eta^{c}_f)=\Td_\phi(\tau_f)\eta^{d}_f.
\end{align}
\todo{Riemann-Roch for refined Gysin.}
Hence, the Todd class measures the difference of fundamental classes in the cohomology theories associated to $\E$ and $\F.$
In fact, $\phi$ induces a \emph{Grothendieck transformation} between $\E^{BM}$ and $\F^{BM}$ in the sense of \cite{fultonCategoricalFrameworkStudy1981}.
\subsection{The Riemann--Roch functor} In the notation of the last section, can use the Todd classes to define the \emph{Riemann--Roch functor}
$$\RR_\phi\colon \Corr_{(\E,c)}(Y/S)\to \Corr_{(\F,d)}(Y/S)$$
which is the identity on objects and on morphisms acts via 
\[\begin{tikzcd}[column sep=large]
	{\Hom_{\Corr_{(\E,c)}(S/B)}(X,Y)} & {\Hom_{\Corr_{(\F,d)}(S/B)}(X,Y)} \\
	{\E^{BM}_{2d_X,d_X}(XY/B)} & {\F^{BM}_{2d_X,d_X}(XY/B)}
	\arrow[from=1-1, to=1-2]
	\arrow[Rightarrow, no head, from=1-1, to=2-1]
	\arrow[Rightarrow, no head, from=1-2, to=2-2]
	\arrow["{z\mapsto \Td_\phi(\tau_{f_Y})\inv\phi_*(z)}"', from=2-1, to=2-2]
\end{tikzcd}\]
where $f_Y:Y\to B$ is the projection. 
\begin{theorem} The assignment $\RR_\phi$ is a functor, that is, maps the identity to the identity and is compatible with composition.
\end{theorem}
\begin{proof}
One way to proof this statement is by directly using the definition of composition of correspondences and repeatedly applying the Riemann--Roch theorem.
The second way is to show that the following diagram commutes 
\[\begin{tikzcd}
	{\Corr_{(\E,c)}(Y/S)} & {\Corr_{(\E,c)}(Y/S)} \\
	\DE\E & \DE\F
	\arrow["{\phi_*}", from=2-1, to=2-2]
	\arrow["{\Ff_{(\E,c)}}"', from=1-1, to=2-1]
	\arrow["{\RR_\phi}", from=1-1, to=1-2]
	\arrow["{\Ff_{(\F,c)}}", from=1-2, to=2-2]
\end{tikzcd}\]
and to use that the vertical arrows are fully faithful. This boils down to show that the following diagram is commutative
\[\begin{tikzcd}[column sep = 50pt]
	{\E^{BM}_{2d_X,d_X}(XY/B)} & {\F^{BM}_{2d_X,d_X}(XY/B)} \\
	{\E^{BM}_{0,0}(XY/Y)} & {\F^{BM}_{0,0}(XY/Y)}
	\arrow["{\Td_\phi(\tau_{f_Y})\inv\phi_*}", from=1-1, to=1-2]
	\arrow["{\delta_{f_Y}^{(\E,c)}}", from=2-1, to=1-1]
	\arrow["{\delta_{f_Y}^{(\F,d)}}"', from=2-2, to=1-2]
	\arrow["{\phi_*}", from=2-1, to=2-2]
\end{tikzcd}\]
Since $\delta_{f_Y}^{(\E,c)}$ and $\delta_{f_Y}^{(\F,d)}$ arise from multiplication with $\eta_{f_Y}^{(\E,c)}$ and $\eta_{f_Y}^{(\F,d)},$ respectively, this follows from \eqref{eq:toddclassandfundamentalclasses}.
\end{proof}
The Riemann--Roch functor extends to pure motives in the obvious way and we obtain the following.
\begin{corollary}
There is a commutative diagram of functors
\[\begin{tikzcd}
	{\Pure_{(\E,c)}(S/B)} & {\Pure_{(\F,d)}(S/B)} \\
	{\ho\DE{\E}(S)} & {\ho\DE{\F}(S)}
	\arrow["{\Ff_{(\E,c)}}"', from=1-1, to=2-1]
	\arrow["{\phi_*}"', from=2-1, to=2-2]
	\arrow["{\RR_\phi}", from=1-1, to=1-2]
	\arrow["{\Ff_{(\F,d)}}"', from=1-2, to=2-2]
\end{tikzcd}\]
\end{corollary}
\begin{corollary}
	Under the assumptions of \cref{thm:existenceofweightstructure} for $\E$ and $\F$ and assuming additionally that $\phi_*$ is weight exact, we obtain the commutative diagram of functors
\[\begin{tikzcd}
	{\DE{\E}_{(S/B)\! \op{-c}}(S)} & {\Ch^b(\ho\DE{\E}_{(S/B)\! \op{-c}}(S)^{w=0})} & {\Ch^b(\Pure_{(\E,c)}(S/B))} \\
	{\DE{\F}_{(S/B)\! \op{-c}}(S)} & {\Ch^b(\ho\DE{\F}_{(S/B)\! \op{-c}}(S)^{w=0})} & {\Ch^b(\Pure_{(\F,d)}(S/B)).}
	\arrow[from=1-1, to=1-2]
	\arrow["{\Ff_{(\E,c)}\inv}", from=1-2, to=1-3]
	\arrow["{\phi_*}"', from=1-1, to=2-1]
	\arrow["{\phi_*}"', from=1-2, to=2-2]
	\arrow["{\RR_\phi}", from=1-3, to=2-3]
	\arrow["{\Ff_{(\F,d)}\inv}"', from=2-2, to=2-3]
	\arrow[from=2-1, to=2-2]
\end{tikzcd}\]
\end{corollary}

\section{Equivariance via limit extension}
We explain how to extend the previous discussion to quotient stacks $\Xx=[X/G].$
\subsection{Limit extensions of a bivariant formalism}
\subsection{Limit extensions of a motivic triangulated category}
\subsection{The equivariant Riemann--Roch functor}

\section{Motives and $K$-motives}
We apply our discussions in the example of $\DM$ and $\DK.$
\subsection{Construction of ($K$-)motives}
\subsection{Riemann--Roch functor for ($K$-)motives}
\subsection{Example: The Iwahori--Hecke algebra}
